# Supplementary material for: Real-Time Neural Hair G-Buffer Anti-Aliasing
Source: arXiv:2605.17557 source file (2026-08-31)
Supplement: Supplementary file 1 [file Supplement_appendix.tex]

\clearpage
\newpage

\section{Some reflections}

\textbf{Why perform denoising in the GBuffer space instead of color space?}

Operating in GBuffer space decouples geometric reconstruction from shading, making it possible to resolve structural artifacts caused by sparse sampling and visibility changes before color integration. This separation significantly reduces the risk of temporal or spatial oversmoothing of high-frequency hair features.

Compared to GBuffer geometric features, color signals are generally more continuous and smooth in spatial distribution, more in line with the regression hypothesis of neural networks. However, color indicates that geometry, material, and lighting information are highly coupled at the same time, lack clear physical interpretability, and have the problem of irreversible information and ambiguity.

\textbf{Why NN fail to predict position?}

Predicting position requires the network to reconstruct absolute geometry, whereas tangent and coverage only encode local or differential properties, making position regression fundamentally harder.

Even given the denoised strand tangent as a first-order differential constraint and the denoised depth as a 1D projection along the view ray, the hair position still cannot be uniquely determined. Instead, these constraints define a low-dimensional family of feasible positions. A neural network can exploit this structure to only estimate a probabilistic or proxy position consistent with both tangent continuity and depth observations, rather than attempting exact geometric reconstruction.

\textbf{What is predicting position from tangent?}

It's analogous to reconstructing a distribution from its first-order derivatives. 
$$
P(s) = (x(s), y(s), z(s)),s \in [0,1]
$$
where $s$ denotes the arc-length parameter along the strand.
The tangent vector of the curve is defined as
$$
t(s) = \frac{d(P(s))}{ds}.
$$
If the tangent field is known, the curve can be recovered by integrating the tangent vector along the strand:
$$
P(s) = P_0 + \int^s_0 t(u)du,
$$
where $P_0$ denotes an anchor point on the curve.

\textbf{Why denoise in temporal in addition to spatial domain}

In spatial denoising, we mainly rely on the geometry prior learned by the neural network to replace spatial multi-sampling. 
In temporal denoising, we have jittered sampling in the history frames, which are accumulated as a temporal multi-sampling to the current spatial distribution, mitigating the noisy caused by spatial undersampling.
Our network further learns the prior of how to arrange the spatial samplings.
