# Supplementary material for: Real-Time Neural Hair G-Buffer Anti-Aliasing
Source: arXiv:2605.17557 source file (2026-08-31)
Supplement: Supplementary file 2 [file Table_static_supplementary.tex]

\begin{table}[hbt]
\centering
\small
\caption{Masked-hair metrics of static scene for row 2~4 in Fig. 4 in the main paper.} 
\label{tab:sup_static_three}
\renewcommand{\tabcolsep}{0.15cm}
\begin{tabular}{clccccc}
\toprule
& Method 
& MSE$\downarrow$ 
& PSNR$\uparrow$ 
& SSIM$\uparrow$ 
& LPIPS$\downarrow$ 
& FLIP$\downarrow$ \\
\midrule

\multirow{7}{*}{\rotatebox{90}{Ponytail}}
& Input & 0.035698 & 14.47 & 0.9209 & 0.0762 & 0.0569 \\
& MSAA  & 0.006298 & 22.01 & 0.9611 & 0.0243 & 0.0189 \\
& SSAA  & 0.016119 & 17.93 & 0.9426 & 0.0465 & 0.0408 \\
& TAA   & 0.017470 & 17.58 & 0.9478 & 0.0373 & 0.0449 \\
& FSR   & 0.017276 & 17.63 & 0.9435 & 0.0396 & 0.0428 \\
& DLSS  & 0.013619 & 20.43 & 0.9502 & 0.0329 & 0.0388 \\
& Ours  & \textbf{0.001451} & \textbf{28.38} & \textbf{0.9861} & \textbf{0.0058} & \textbf{0.0096} \\

\midrule

\multirow{7}{*}{\rotatebox{90}{Straight}}
& Input & 0.016397 & 17.85 & 0.8603 & 0.1226 & 0.0751 \\
& MSAA  & 0.014004 & 18.54 & 0.8870 & 0.0678 & 0.0728 \\
& SSAA  & 0.007698 & 21.14 & 0.8971 & 0.0844 & 0.0528 \\
& TAA   & 0.006899 & 21.61 & 0.9136 & 0.0687 & 0.0593 \\
& FSR   & 0.007417 & 21.30 & 0.9066 & 0.0671 & 0.0581 \\
& DLSS  & 0.005835 & 22.34 & 0.9175 & 0.0543 & 0.0521 \\
& Ours  & \textbf{0.000644} & \textbf{30.91} & \textbf{0.9812} & \textbf{0.0083} & \textbf{0.0143} \\

\midrule

\multirow{7}{*}{\rotatebox{90}{Afro}}
& Input & 0.031836 & 14.97 & 0.9295 & 0.0573 & 0.0173 \\
& MSAA  & 0.006471 & 21.89 & 0.9264 & 0.0578 & 0.0168 \\
& SSAA  & 0.017715 & 17.52 & 0.9000 & 0.0932 & 0.0291 \\
& TAA   & 0.010190 & 19.92 & 0.9347 & 0.0591 & 0.0283 \\
& FSR   & 0.012383 & 19.07 & 0.9218 & 0.0772 & 0.0289 \\
& DLSS  & 0.009815 & 20.08 & 0.9338 & 0.0583 & 0.0289 \\
& Ours  & \textbf{0.001805} & \textbf{26.43} & \textbf{0.9659} & \textbf{0.0206} & \textbf{0.0073} \\

\bottomrule
\end{tabular}
\end{table}
